# Supplementary material for: Understanding the Stability of Deep Control Policies for Biped Locomotion
Source: arXiv:2007.15242 source file (2020-07-30)
Supplement: Supplementary file 1 [file supplementary.tex]

% Appendix
% \appendix

% \pagebreak
\section*{Supplementary Material}

\color{red} 앞으로 옮기자! \color{black}

\begin{alphasection}

\section{DRL controller training list}

We trained 8 biped controllers using DRL based on a combination of the following four options: 

\begin{itemize}
  \item All crouch motions / Each crouch motion
  \item with push / without push 
  \item Uniform sampling / Adaptive sampling
%   \item Joint torque model / Musculoskeletal model
\end{itemize}

% Default setup : joint-torque model with simple foot model, All variation (crouch angle, step length, and walking speed), training with push.
% We conducted same set of experiment above, but using different combination of character models and foot models described below.

% \paragraph{Character model.}

% \begin{itemize}
%   \item musculoskeletal model + multi-segment foot model
%   \item musculoskeletal model + simple foot  model
%   \item joint-torque model + multi-segment foot model
%   \item joint torque model + simple foot model
% \end{itemize}

\section{Push recovery experiment dataset for comparison with human data}

Ten thousand push recovery experiments were performed for each level of crouch on each controller.
The number of successful tuples in each category is shown in Table ~\ref{tab:appendix_data}.

% 각 컨트롤러의 각 level of crouch (0, 20, 30, 60)마다 만 개씩 push recovery experiment를 수행하였다.
% 고서 성공한 tuple data들을 사용하였다.  
% 표에는 각 카테고리마다 성공한 tuple들의 개수를 적어놓았다.

\definecolor{Gray}{gray}{0.9}
\begin{table*}
% \begin{center}
\centering
    \begin{tabular}{lclclclclclclclclclcl}
      \toprule
     Sampling &    Motion &    Push    &  Normal & crouch20 & crouch30 & crouch60 & Group 1 & Group 2 & Total   \\
    \midrule
              &  All  &    o    &   682    &  1273    &  2317  &  2511   &  1748   &  6783    &  6783   \\
              \rowcolor{gray}
     Uniform  &  One  &    o    &   3561   & 5006     &  5685  &  3483   &  3727      &  17735    &   17735   \\
              &  All  &    x    &    27    &    64    &  75    &   41    &   45    &   207   &    207    \\
              &  One  &    x    &    33    &    76    &  280   &   754   &   404   &   929   &  1143    \\
     \midrule
            %   &  All  &    o    &        &     &    &     &     &    &       \\
     Adaptive &  One  &    o    &   3546    &   4079  & 5732   &    4639     &   4089   &  17996    &    17996    \\
            %   &  All  &    x    &       &     &    &     &     &    &       \\
            %   &  One  &    x    &       &     &    &     &     &    &       \\
    %  \midrule

    %                     &          &  All  &    o    &  437   & 1982 & 1751 & 64    &  2640   &    4234  &  4234       \\
    %  Musculoskeletal    &  Uniform &  One  &    o    &  2537  & 3069 & 4174 & 158   &  2346   & 9938     & 9938        \\
    %     model           &          &  All  &    x    &  91    & 736  & 903  &  14   &  645 &  1744  &  1744  \\
    %                     &          &  One  &    x    & 123    & 237  & 158  &  618  &  386   & 1136 & 1136  \\
    %   \midrule
    %                     &          &  All  &    o    &       &     &    &       &     &      &         \\
    %  Musculoskeletal    & Adaptive &  One  &    o    &       &     &    &       &     &      &         \\
    %     model           &          &  All  &    x    &  28   &     &    &       &     &      &        \\
    %                     &          &  One  &    x    &       &     &    &       &     &      &       \\
      \bottomrule
    \end{tabular}
% \end{center}
\bigskip\centering
\caption{The number of successful experimental data we used. Default controller is shown in gray.}
\label{tab:appendix_data}
\end{table*}%

\section{Push recovery experiment dataset for comparison between Drl controllers}

For the constant push force (100N), 1,000 experiments were performed for each level of crouch on each DRL controller.
% We conducted one thousand experiments for each DRL controller. 

% Table
\begin{table*}
% \begin{center}
\centering
    \begin{tabular}{lclclclclclclclclclcl}
      \toprule
        Motion  &    Push    &  Normal & crouch20 & crouch30 & crouch60 &   Total   \\
    \midrule
                &  All  &    o    &   338  & 546   & 535  &  222  &  1641   \\
                \rowcolor{gray}
     Uniform    &  One  &    o    &   625  & 667   & 720  &  538  &  2550   \\
                &  All  &    x    &  260   &  221  & 111  &  94  &   686   \\
                &  One  &    x    &  26    &  124  & 313  &  470  &  933   \\
     \midrule
                &  All  &    o    &  507   &  788  & 719  &  478  &  2492   \\
      Adaptive  &  One  &    o    &  802   &  704  & 787  &  755  &  3048   \\
                % &  All  &    x    &     &    &   &    &     \\
                % &  One  &    x    &     &     &   &    &     \\
    %  \midrule

    %                     &          &  All  &    o    &   &    &   &    &     \\
    %  Musculoskeletal    &  Uniform &  One  &    o    &   &    &   &    &     \\
    %     model           &          &  All  &    x    &   &    &   &    &     \\
    %                     &          &  One  &    x    &   &    &   &    &     \\
    %   \midrule
    %                     &          &  All  &    o    &     &    &   &    &     \\
    %  Musculoskeletal    & Adaptive &  One  &    o    &     &    &   &    &     \\
    %     model           &          &  All  &    x    &     &    &   &    &     \\
    %                     &          &  One  &    x    &     &    &   &    &     \\
      \bottomrule
    \end{tabular}
% \end{center}
\bigskip\centering
\caption{The number of successful experimental data we used for the constant force (100N). Default controller is shown in gray.}
\label{tab:appendix_data_drl}
\end{table*}%

\end{alphasection}
